# Supplementary material for: Interpretable Neuron Structuring with Graph Spectral Regularization
Source: arXiv:1810.00424 source file (2020-02-14)
Supplement: Supplementary file 1 [file supplement.tex]

\section{Experiment Specifics}
We use Leaky relus with a coefficient of 0.2 \cite{maas2013rectifier} for all layers except for the embedding and output layers unless otherwise specified. We use the ADAM optimizer with default parameters \cite{kingma2014adam}.

\paragraph{Laplacian Smoothing on an Autoencoder}
We use an autoencoder with five fully connected layers for the hierarchical example. The layers have widths [50,50,6,50,50]. To perform Laplacian smoothing on this autoencoder we add a term to the loss function. Let $\nu$ be the activation vector on the embedding layer, then we add a penalty term $\alpha \nu^T L \nu$ where $\alpha$ is a weighting hyperparameter to the standard mean squared error loss. For the biological example the layers have widths [50,50,20,50,50]. When not otherwise mentioned we use a graph spectral regularization strength of $\alpha = 0.001$.

\begin{table}[h]
\centering
\subfloat[Basic MNIST classifier used with and without Laplacian smoothing on layer 5.]{
\scalebox{0.9}{\begin{tabular}{|l|l|l|l|l|}
\hline
\# & type          & patch/stride & depth & output size \\ \hline\hline
1  & convolution   & 5x5/1        & 32    & 28x28x32    \\ \hline
2  & max pool      & 2x2/2        &       & 14x14x32    \\ \hline
3  & convolution   & 5x5/1        & 64    & 14x14x64    \\ \hline
4  & max pool      & 2x2/2        &       & 7x7x64      \\ \hline
5  & dense         &              & 64    & 8x8         \\ \hline
6  & dense         &              & 10    & 1x10        \\ \hline
\end{tabular}}\label{tab:basic}}
\hfill
\subfloat[MNIST classifier structure with convolutions following the Laplacian smoothing layer (layer 6).]{
\scalebox{0.9}{\begin{tabular}{|l|l|l|l|l|}
\hline
\# & type          & patch/stride & depth & output size \\ \hline\hline
1  & convolution   & 5x5/1        & 32    & 28x28x32    \\ \hline
2  & max pool      & 2x2/2        &       & 14x14x32    \\ \hline
3  & convolution   & 5x5/1        & 64    & 14x14x64    \\ \hline
4  & max pool      & 2x2/2        &       & 7x7x64      \\ \hline
5  & dense         &              & 64    & 8x8         \\ \hline
6  & convolution   & 3x3/1        & 16    & 8x8x16      \\ \hline
7  & max pool      & 2x2/2        &       & 4x4x16      \\ \hline
8  & convolution   & 3x3/1        & 16    & 4x4x16      \\ \hline
9  & max pool      & 2x2/2        &       & 2x2x16      \\ \hline
10 & convolution   & 3x3/1        & 16    & 2x2x16      \\ \hline
11 & dense         &              & 10    & 1x10        \\ \hline
\end{tabular}}
\label{tab:conv}}
\caption{Structure of MNIST classifiers with Laplacian smoothing}
\end{table}

\paragraph{MNIST Classifier Architecture}
The basic classifier that we use consists of two convolution and max pooling layers followed by the dense layer where we apply Laplacian smoothing. We use the cross entropy loss to train the classification network in this case. Note that while we use convolutions before this layer for the MNIST example, in principle, techniques applied here could be applied to non image data by using only dense layers until the Laplacian smoothing layer which constructs an image for each datapoint. Table~\subref*{tab:basic} shows the architecture when no convolutions are used. Table~\subref*{tab:conv} exhibits the architecture when convolution and max pooling layers are used after the Laplacian smoothing layer constructs a 2D image.
